# Supplementary material for: Adaptive Rejection of Periodic Disturbances Acting on Linear Systems with Unknown Dynamics
Source: arXiv:1603.05361 source file (2016-03-17)
Supplement: Supplementary file 1 [file apndx-proof-directadaptive.tex]

\section{Proof of Theorems }
We use the method of analysis of stochastic recursive
algorithms discussed in \cite{ljung1977analysis} to study the
convergence and asymptotic behavior of the proposed adaptive algorithm with
the update rule given in \eqref{eq:paa}.
The key idea is that a differential equation counterpart 
for \eqref{eq:paa} is derived and it is shown that
the only convergence point of \eqref{eq:paa} is the 
stable equilibrium of this differential equation.
Moreover, it is shown that the estimated parameters
 converge with probability one to this equilibrium under
some mild assumptions on the excitation signal power or initial 
values of parameters.

\subsection{Preliminaries}
A general recursive algorithm can be formalized as
\begin{align}\label{eq:paa-general}
\hat{\Theta}(k)=\hat{\Theta}(k-1)+ \gamma(k)Q(k;\hat{\Theta}(k-1), \Phi(k))
\end{align}
where $\hat{\Theta}(k)\in \R^n$ is a sequence of $n$-dimensional column vectors
referred as  ``the estimates''. In our particular recursive algorithm, they stand for
the parameters of system dynamics in conjunction with the parameters that determine the adaptive control law.
$\gamma(k)$ is assumed to be
a sequence of positive scalars. The $m$-dimensional vector
$\Phi(k)$ is an observation obtained at time $k$ which is usually called the ``regressor''. The information
contained in $\Phi(k)\in \R^m$ sequence cause $\hat{\Theta}(k-1)$ to be updated.
The map $Q(.;.,.)$ from $R\times R^n \times R^m$ into $R^n$ is a
deterministic function with some regularity conditions that 
guarantee the convergence of the adaptive algorithm to 
some ``desired'' points that will be discussed later. 
%From the above equation it can be inferred that 
%$Q(.;.,.)$ together with the choice
%of the ``gain'' sequence $\gamma(.)$ determine entirely the
%algorithm.

The regressor vector $\Phi(k)$ is, in general, a function of the
previous measurements (when the system has memory), the 
previous estimates (when the estimates define an adaptive control law),  
and the inputs to the system (all other control signals and noises).
A very broad class of update rules, as of ours, can be realized by a 
time varying linear system
\begin{align*}
\Phi(k)= A_{\Phi}(\hat{\Theta}_{k-1}) \Phi(k-1) + B_{\Phi}(\hat{\Theta}_{k-1}) U(k)
\end{align*}
where $A_{\Phi}$ and $B_{\Phi}$ are $m\times m $ and $m\times r$ matrix functions and $U(k)\in \R^r$ stands for all control signals and noises entering the system.

In a stochastic framework, $Q(k;\hat{\Theta}(k-1), \Phi(k))$ is a random variable. This implies that
convergence can take place only if the noise is rejected by paying less
attention to the observations as time passes, i.e. by letting
\begin{align*}
\gamma(k)\rightarrow 0 \qquad \text{as}~~ k\rightarrow \infty.
\end{align*}
However, this is not feasible when the actual (system) parameters are time-varying, as in 
tracking problems. 
For such problems, $\gamma(k)$ can tend to very small, but still positive, values and 
the analysis carried out in this section will give some insights regarding the
algorithm behavior.

The estimated parameters and the regressor in our adaptive algorithm are
	\begin{align*}
		&\hat{\Theta}(k):=\begin{bmatrix} \tha_A(k) \\ \tha_B(k) \\ \tha_C(k) \\ \tha_M(k)  \\ \text{col}\left[F(k)\right] \\ f(k) \end{bmatrix}
		&\Phi(k):= 
		\left[\begin{array}{c}
		\phi_{e}(k) \\ \hdashline u(k) \\ \phi_u(k) \\ \hdashline {\bar{w}}(k) \\\phi_{\bar{w}}(k) \\ \hdashline \phi_{\epsilon}(k) \\\hdashline \phi_R(k) \\\hdashline \phi_{ u_{A}}(k)
		\end{array} \right].
	\end{align*}
where $\text{col}[x]$ of a matrix $x$ refers to a vector created by stacking the columns of matrix $x$.
The $A_{\Phi}$ and $B_{\Phi}$ matrix functions can be written as

	\begin{widetext}
		\begin{align}\label{eq:A}
		A_{\Phi}(\hat{\Theta}_{k-1}):=
		{\tiny
			\left[\begin{array}{cccccccc}
			\theta_A^T  & \begin{bmatrix} 0 & \theta_B^T \end{bmatrix} & \begin{bmatrix} 0 & \theta_C^T  \end{bmatrix}& 0_{n_A} & \theta_R^T & \theta_B^T \\ 
			\begin{bmatrix} I_{n_A-1} & 0 \end{bmatrix} &0 &0 &0 &0 &0 \\\hdashline 
			0 & \begin{bmatrix} 0 & 0\\I_{n_A} & 0   \end{bmatrix} &0 &0 &0 &0 \\ \hdashline
			0 & 0  & \begin{bmatrix} 0 & 0 \\I_{n_A} & 0  \end{bmatrix} & 0 &0 &0 \\ \hdashline
			\hat{\theta}_A^T(k-1)& \begin{bmatrix} 	0 & \hat{\theta}_B^T(k-1) \end{bmatrix} &0 &\hat{\theta}_C^T(k-1) &\hat{\theta}_M^T(k-1) &0 \\
			0 & 0 & 0 & \begin{bmatrix} I_{n_A-1	} & 0  \end{bmatrix}  &0 &0 \\ \hdashline
			0 & 0 & 0 & 0 & 0  &0 \\ \hdashline
			0 &0 &0 &0 &\hat{\theta}_D^T(k-1) &0 \\ 
			0 & 0 & 0 &0 &0 &\begin{bmatrix} I_{n_A-1} & 0  \end{bmatrix} 
			\end{array} \right]}
		\end{align}
	\end{widetext}
% B
	\begin{align}\label{eq:B}
		B_{\Phi}(\hat{\Theta}_{k-1}):=
		\left[\begin{array}{ccc}
		0 & 0 &0\\\hdashline
		\begin{bmatrix} I \\ 0 \end{bmatrix} &0 &0\\\hdashline
		0& \begin{bmatrix} I \\ 0 \end{bmatrix} &0\\\hdashline
		0 & 0 &0\\\hdashline	
		0& 0& \begin{bmatrix} I \\ 0 \end{bmatrix} \\\hdashline
		0 & 0 &0	
		\end{array} \right]
		\end{align}
		and the input vector is
		\begin{align}\label{eq:U}
		U(k):=
		\left[\begin{array}{c}
		u(k)\\{\bar{w}}(k)\\\phi_R(k)
		\end{array} \right].
	\end{align}
The next part provides certain regularity
conditions on functions $Q$,  $A_{\Phi}$ and $B_{\Phi}$ as well as
driving ``input'' term $U$ to analyze the behavior of \eqref{eq:paa-general}.
Before that, we provide two Lemmas about Lipschitz continuity (LC) properties of real valued functions since these results will be used in the sequel. The proofs of both lemmas can be found in \cite{eriksson2013applied}.
\begin{lemma}[LC of product of functions]\label{lem:lcprod}
	$f(x)={f_1(x)}{f_2(x)}$ is Lipschitz continuous on a bounded set $I$ if $f_1(.)$ and $f_2(.)$ are individually Lipschitz continuous on the same set.
\end{lemma}
\begin{lemma}[LC of quotient of functions]\label{lem:lcquotient}
	$f(x)=\frac{f_1(x)}{f_2(x)}$ is Lipschitz continuous on a bounded set $I$ if $f_1(.)$ and $f_2(.)$ are individually Lipschitz continuous on the same set and there is a positive constant $m$ such that for any $x\in I$, $f_2(x)\ge m$.
\end{lemma}

\subsection{Regularity Conditions}
Three sets of regularity conditions are proposed in \cite{ljung1977analysis} to
analyze a recursive algorithm in the form of \eqref{eq:paa-general}.
The first two sets, referred as ``Assumptions A'' and ``Assumptions B'', 
consider $U(k)$ as a sequence of random variables and treat the algorithm in a stochastic framework.
In our method, the input signal $U(k)$ \eqref{eq:U} is consisted of stochastic and deterministic parts, e.g. $\Phi_R(k)$ is a known vector whereas $\bar{w}(k)$ is a random sequence.
The third set of assumptions referred as ``Assumptions C'' is more general and will be used here.
Let $\mathscr{D}_S(x)$ be the set of all $A_{\Phi}(x)$ that have all eigenvalues strictly inside the unit circle and 
let $\mathscr{D}_R$ be an open connected subset of $\mathscr{D}_S(x)$. ``Assumptions C'' in \cite{ljung1977analysis} are given in the following.

%=============================================================================================
\subsubsection{Assumptions C}\label{ass:c}
\begin{enumerate}
	\item \label{ass:c1} The function $Q\left(k,x,\phi\right)$ is Lipschitz continuous in $x$ and $\phi$. In other words, 
	$|Q\left(k,x_1,\phi_1\right)-Q\left(k,x_2,\phi_2\right)|<\mathscr{K}\left(x,\phi,\rho, \nu\right)\left\{|x_1-x_2|+|\phi_1-\phi_2|\right\}$ 
	for any $x_1$ and $x_2$ in $\mathscr{B}(x,\rho(x))$ ($\mathscr{B}(x,\rho)$ denotes a $\rho$-neighborhood of $x$) for some $\rho(x)>0$ where $x\in \mathscr{D}_R$. Moreover, $\phi_1$ and $\phi_2$ should be in $\mathscr{B}\left(\phi, \nu \right)$ for some $\nu \ge 0$.
	\item \label{ass:c2} The matrix functions $A_{\Phi}(x)$ and $B_{\Phi}(x)$ are \lc\ in $x$.
	\item \label{ass:c3} $z(k,\bar{x})$ as defined by $z(0,\bar{x})=0$ and 
		\begin{align}\label{eq:z}
			\begin{split}
			&z(k,\bar{x})=z(k-1,\bar{x})+\\
			&\qquad \quad \gamma(k)\left[Q(k,\bar{x},\bar{\phi}(k,\bar{x}))-z(k-1,\bar{x})\right] \\
			\end{split}
		\end{align}
	converges for all $\bar{x}\in\mathscr{D}_R$ as $k\rightarrow \infty$. Denote the limit by $\mathscr{F}(\bar{x})$.
	\item \label{ass:c4} $k_v(k,\bar{x},\lambda,c)$ defined by $k_v(0,\bar{x},\lambda,c)=0$ and 
		\begin{align}\label{eq:kv}
		\begin{split}
			&k_v(k,\bar{x},\lambda,c) = k_v(k-1,\bar{x},\lambda,c)+\\
			&\quad \gamma(k) \left[\mathscr{K}\left(\bar{x},\bar{\phi}(k,\bar{x}),\rho(\bar{x}),\nu(k,\lambda,c)\right) \right. \\
			&\quad \quad 
			\cdot\left.
			\left(1+\nu(k,\lambda,c)\right)-k_\nu (k-1,\bar{x},\lambda,c)
			\right]
		\end{split}
		\end{align}
	converges to a finite limit as $k\rightarrow \infty$ for all $\bar{x}\in \mathscr{D}_R$, $\lambda<1$ and $c<\infty$.
	\item \label{ass:c5} $\sum\limits_{k=1}^{\infty}\gamma(k)=\infty$.
	\item \label{ass:c6} $\gamma(k)\rightarrow 0$ as $k\rightarrow \infty$.
\end{enumerate}

\paragraph*{Assumption \ref{ass:c1}:} The function $Q(k;\hat{\Theta}(k-1),\Phi(k))$ in \eqref{eq:paa-general} in our algorithm is time invariant. We abuse the notation and use $Q(\hat{\Theta}(k-1),\Phi(k))$ in the sequel. This function can be written as
	\begin{align}
		\label{eq:Q}
		&Q\left(\hat{\Theta}(k-1), \Phi(k) \right):= \begin{bmatrix}Q_1(\hat{\Theta}(k-1), \Phi(k))\\Q_2(\hat{\Theta}(k-1), \Phi(k))\\Q_3(\hat{\Theta}(k-1), \Phi(k))\end{bmatrix}
	\end{align} 
where
	\begin{align}
		\label{eq:Q1}
		&Q_1(\hat{\Theta}(k-1), \Phi(k)):= \bm{cc} F^{-1}(k-1) & 0 \\ 0 & f^{-1}(k-1)I \mb
		\\ \notag
		&\qquad\quad  \cdot M_1 \Phi(k)\left(M_3^T \Phi(k)- M_2\hat{\Theta}^T(k-1)M_1\Phi(k)\right) 
		\\
		\label{eq:Q2}
		&Q_2(\hat{\Theta}(k-1), \Phi(k)):= \text{Col}\left\{ M_4   \Phi(k)\Phi^T(k) M_4^T - F(k-1) \right\}
		\\
		\label{eq:Q3}
		&Q_3(\hat{\Theta}(k-1), \Phi(k)):=  \Phi(k)^T M_5^T M_5 \Phi(k) - f(k-1)
	\end{align}
and the matrices $M_1$, $M_2$, $M_3$, $M_4$ and $M_5$ are defined as follows
	\begin{align}
	\notag 
	\phi(k):&=\begin{bmatrix}\phi_{e}(k) \\ \phi_u(k)\\ \phi_{\epsilon}(k) \\ \phi_R(k) \end{bmatrix}=\underbrace{\begin{bmatrix}
		\text{diag}\bk{ccccccc} I  & \begin{bmatrix} 0& I \end{bmatrix} & \begin{bmatrix} 0& I \end{bmatrix}&I  \kb
		& 0	\end{bmatrix}}_{M_1} \Phi(k)
	\\
	\notag
	\hat{\theta}(k):&=\begin{bmatrix}\tha_A(k)\\ \tha_B(k) \\ \tha_C(k) \\ \tha_M(k) \end{bmatrix} = \underbrace{\begin{bmatrix}
		I & 0
		\end{bmatrix}}_{M_2} \hat{\Theta}(k)
	\\
	\notag
	{e}(k)&= \underbrace{\left[\begin{array}{cccccccc}
		\theta_A^T  & \begin{bmatrix} 0 & \theta_B^T \end{bmatrix} & \begin{bmatrix} 0 & \theta_C^T  \end{bmatrix}& 0 & \theta_R^T & \theta_B^T 	\end{array} \right]}_{M_3^T} \Phi(k)
	\\
	\notag
	\begin{bmatrix}\phi_{e}(k) \\ \phi_u(k)\\ \phi_{\epsilon}(k)  \end{bmatrix}&=\underbrace{\begin{bmatrix}
		\text{diag}\bk{ccccccc} I  & \begin{bmatrix} 0& I \end{bmatrix} &\begin{bmatrix} 0& I \end{bmatrix} \kb & 0
		\end{bmatrix}}_{M_4} \Phi(k) 
	\\
	\notag
	\phi_R(k) &=\underbrace{\bm{ccccccc} 0   &I & 0\mb}_{M_5} \Phi(k).
	\end{align}
The dimensions of identity and all zero matrices are omitted since they can be determined from the 
regressor and estimated parameters dimensions. 
Equation \eqref{eq:Q} shows that $Q(x,\phi)$ is Lipschitz continuous if $Q_1(x,\phi)$, $Q_2(x,\phi)$ and $Q_3(x,\phi)$ are all \lc. This can be shown by ``triangle inequality''
	$$|Q(x,\phi)|\le |Q_1(x,\phi)|+|Q_2(x,\phi)|+|Q_2(x,\phi)|$$
which implies that
	\begin{align*}
	&|Q(x_1,\phi_1) - Q(x_2,\phi_2) | \\ & \qquad \qquad \le \left(\mathscr{K}_1+\mathscr{K}_2+\mathscr{K}_3\right) \left\{|x_1-x_2|+|\phi_2 - \phi_2|\right\}
	\end{align*}
where $\mathscr{K}_1$, $\mathscr{K}_2$ and $\mathscr{K}_3$ are the Lipschitz constants of $Q_1(.,.)$, $Q_2(.,.)$ and $Q_3(.,.)$ in a bounded region of interest. With the same argument, we can claim that each $Q_i$ -- as a vector valued function -- is \lc\ if each of its individual components is \lc. Equations \eqref{eq:Q2} and \eqref{eq:Q3} show that $Q_2(.,.)$ and $Q_3(.,.)$ are always \lc\ by Lemma~\ref{lem:lcprod}. Moreover, $Q_1(.,.)$ is \lc\ as long as $F$ is non singular and $f$ is non zero. This can be shown by Lemma~\ref{lem:lcprod} and \ref{lem:lcquotient}, and the fact that matrix inversion incorporates determinants of sub-regions of the original matrix (i.e. cofactors) and inverse of the matrix determinant. It is clear that the cofactor elements are simply polynomials and thus \lc, and the inverse of the matrix determinant is \lc\ by Lemma~\ref{lem:lcquotient} as long as it is always nonsingular in $\mathscr{B}(x,\rho)\times \mathscr{B}(\phi,\nu)$.

\paragraph*{Assumption \ref{ass:c2}:} It is clear that $A_{\Phi}(\hat{\Theta})$ and $B_{\Phi}(\hat{\Theta})$ given by \eqref{eq:A} and \eqref{eq:B} are both (Lipschitz) continuous in $\hat{\Theta}$.

\paragraph*{Assumption \ref{ass:c3}:} By following the same approach as in the proof of Lemma 2 in \cite{ljung1977analysis}, we can show that when the following conditions are satisfied
\begin{enumerate}
	\item Assumption \ref{ass:c1} holds
	\item $\mathscr{K}$ in \ref{ass:c1} is \lc  ~in $\phi$ and $\nu$ 
		\begin{align*}
			&|\mathscr{K}\left(x,\phi_1,\rho,\nu_1 \right)
			-\mathscr{K}\left(x,\phi_2,\rho,\nu_2 \right)|
			\le  \\
			& \qquad \qquad \mathscr{H}\left(x,\phi,\rho,\nu,w \right)\left\{|\phi_1-\phi_2|+|\nu_1-\nu_2|\right\}
		\end{align*}
	for $\phi_1,\phi_2\in \mathscr{B}(\phi,w)$ and $\nu_1,\nu_2\in \mathscr{B}(\nu,w)$
	\item For all $x\in\mathscr{D}_R$, the functions $Q$, $\mathscr{K}$ and $\mathscr{H}$ have bounded $p$-moments for all $p>1$, $\lambda<1$ and $c<\infty$.
\end{enumerate}
we have
\begin{align}\label{eq:sumToExpect}
	\frac{1}{t}\sum\limits_{k=1}^{t} Q\left(\bar{x}, \bar{\phi}(k,\bar{x})\right) \rightarrow \frac{1}{t}\sum\limits_{k=1}^{t} \E \left[Q\left(\bar{x}, \bar{\phi}(k,\bar{x})\right)\right]
\end{align}
with probability one as $t\rightarrow \infty$.
We have already shown that \ref{ass:c1} holds and a \lc~ function $\mathscr{K}$ can be defined. The last condition holds as long as $|F(k)|$ and $|f(k)|$ are non-zero.
This expression \eqref{eq:sumToExpect} with \eqref{eq:z} when $\gamma(k)= 1/k$ imply
\begin{align}\label{eq:sumE}
	z(t,\bar{x})\rightarrow\frac{1}{t}\sum\limits_{k=1}^{t} \E \left[Q\left(\bar{x}, \bar{\phi}(k,\bar{x})\right)\right].
\end{align}
with probability one as $t\rightarrow \infty$.
Therefore, in order to show that regularity condition (C.3) is satisfied, it is enough to prove that the limit
$$\mathscr{F}(\bar{x})=\lim\limits_{t\rightarrow\infty}\frac{1}{t}\sum\limits_{k=1}^{t} \E \left[Q\left(\bar{x}, \bar{\phi}(k,\bar{x})\right)\right]$$
exists.

As we will show in the following part, the stochastic process $Q\left(\bar{x}, \bar{\phi}(k,\bar{x})\right)$ is cyclostationary and the limit is well defined. Here, we assume that the excitation signal is also periodic with contents focused at frequencies different than the periodic disturbance. We take $\bar{\Theta}\in \mathscr{D}_R$ which implies that $A_{\Phi}(\bar{\Theta})$ is stable (i.e. has all eigenvalues strictly inside the unit circle). Since $A_{\Phi}(\bar{\Theta})$ and $B_{\Phi}(\bar{\Theta})$ are time invariant, we can use superposition principle for this linear time invariant system and decompose the response $\Phi(k)=\Phi_s(k)+\Phi_d(k)$ into stochastic, $\Phi_s(k)$, and deterministic, $\Phi_d(k)$, parts
\begin{align}\label{eq:phid}
	\Phi_s(k) &= A_{\Phi}(\bar{\Theta}) \Phi_s(k-1) + B_{\Phi_s}(\bar{\Theta}) {\bar{w}}(k) \\ \label{eq:phs}
	\Phi_d(k) &= A_{\Phi}(\bar{\Theta}) \Phi_d(k-1) + B_{\Phi_d}(\bar{\Theta}) \begin{bmatrix} u(k) \\ \phi_R(k)	\end{bmatrix}
\end{align}
where $B_{\Phi_s}$ and $B_{\Phi_d}$ can be clearly found from \eqref{eq:B}. Note that when $u(k)$ is not periodic and rather it is wide-sense stationary the only required modification is to remove $u(k)$ from the input signal in \eqref{eq:phid} and instead append the input in \eqref{eq:phs} with $u(k)$. The rest of analysis will be very similar in this case.

Since $A_{\Phi}(\bar{\Theta})$ is stable, $\Phi_s(k)$ will converge to a zero mean stationary random vector, denoted by $\bar{\Phi}_s(k, \bar{\Theta})$, with bounded covariance and $\Phi_d(k)$ will converge to $\bar{\Phi}_d(k, \bar{\Theta})$ which is a periodic vector that contains sinusoids with the same frequencies as $\phi_R(k)$ and amplitudes/phase-lags that are related to the magnitude and phase of $$\left(e^{jw_i}I-A_{\Phi}(\bar{\Theta})\right)^{-1}B_{\Phi_d}(\bar{\Theta})e^{jw_i}.$$ 
Again, since $A_{\Phi}(\bar{\Theta})$ is stable, $\bar{\Phi}_d(k, \bar{\Theta})$ is bounded and it implies that ${\Phi}(k)$ will converge to $\bar{\Phi}(k, \bar{\Theta})=\bar{\Phi}_s(k, \bar{\Theta})+\bar{\Phi}_d(k, \bar{\Theta})$. We can now return to \eqref{eq:sumE} and show that 
\begin{align}\label{eq:zh}
	\lim\limits_{t\rightarrow \infty} z(t,\bar{x})=\lim\limits_{t\rightarrow \infty} \frac{1}{t}\sum\limits_{k=1}^{t} \E \left[Q\left(\bar{\Theta}, \bar{\Phi}(k,\bar{\Theta})\right)\right] = h\left(\bar{\Theta}\right)
\end{align}
where $h\left(\bar{\Theta}\right)$ is a bounded and well defined function. Note that
	\begin{widetext}
		\begin{align}\label{eq:EQ}
		\E \left[Q\left(\bar{\Theta}, \bar{\Phi}(k,\bar{\Theta})\right)\right] = 
		\bm{c} 
		\bm{cc} \bar{F}^{-1} & 0 \\ 0 & \bar{f}^{-1}  \mb \E \left\{\bar{\phi}(k, \bar{\Theta}) \left(\bar{y}(k,\bar{\Theta}) - \bar{\theta}^T \bar{\phi}(k, \bar{\Theta})\right)\right\} \\
		\text{\emph{Col}}\left\{ \E\left[\bar{\phi}_1(k,\bar{\Theta}) \bar{\phi}_1^T(k,\bar{\Theta} )\right]  -\bar{F} \right\} \\
		\E \left[ \bar{\Phi}(k, \bar{\Theta})^T M_5^T M_5 \Phi(k) - \bar{f}\right]
		\mb
		\end{align}
	\end{widetext}
and we can show that the limit given in \ref{eq:zh} is well defined for all the three terms on the right hand side. For instance, for the first term we have
	\begin{widetext}
			\begin{align}\label{eq:tmp2}
			\begin{split}
			  \E \left\{\bar{\phi}(k, \bar{\Theta}) \left(\bar{y}(k,\bar{\Theta}) - \bar{\theta}^T \bar{\phi}(k, \bar{\Theta})\right)\right\}  &= \E \left\{\bm{c} \bar{\phi}_1(k,\bar{\Theta}) 
			\\ \phi_R(k) \mb \left(\bar{y}(k,\bar{\Theta}) - \bar{\theta}^T \bar{\phi}(k, \bar{\Theta})\right)\right\}
			\\
			&= \bm{c} \E \left[\bar{\phi}_{1s} (k,\bar{\Theta}) \bar{y}_s(k,\bar{\Theta})\right] +  \bar{\phi}_{1d}(k,\bar{\Theta}) \bar{y}_{d}^T(k,\bar{\Theta}) 
			\\
			\phi_R(k) \bar{y}_d(k,\bar{\Theta}) \mb \\
			&\qquad	  - \bm{c} \bar{\theta_1}^T \E \left[\bar{\phi}_{1s} (k,\bar{\Theta}) \bar{\phi}_{1s}(k,\bar{\Theta})\right]+ \bar{\theta_1}^T \bar{\phi}_{1d}(k,\bar{\Theta}) \bar{\phi}_{1d}^T(k,\bar{\Theta}) + \bar{\theta}_M^T \phi_R(k)\bar{\phi}_{1,d} (k,\bar{\Theta}) \\
			\phi_R(k) \bar{\Phi}_d^T(k,\bar{\Theta})\bar{\theta} \mb
			\end{split}
			\end{align}
	\end{widetext}
where $\bar{\phi}_{1s}(.,.):=M_4\bar{\Phi}_s(.,.)$, $\bar{\phi}_{1d}(.,.):=M_4\bar{\Phi}_d(.,.)$ and $\bar{\theta}_1^T:=\begin{bmatrix}\bar{\theta}_A^T & \bar{\theta}_B^T & \bar{\theta}_C^T\end{bmatrix}$. Similarly, $\bar{y}_d(.,.)$ and $\bar{y}_s(.,.)$ are the values corresponding to $y$ respectively in $\bar{\Phi}_d(.,.)$ and $\bar{\Phi}_s(.,.)$. Note that all the stochastic terms will be stationary when $t\rightarrow\infty$ and all deterministic terms become periodic in steady state. Therefore, all the terms in \eqref{eq:tmp2} when plugged to \eqref{eq:zh} produces well defined limits. Following the same type of analysis, it is easy to show that the second and third terms of \eqref{eq:EQ} generate bounded limits when plugged to \eqref{eq:zh}.

\paragraph*{Assumptions \ref{ass:c4}:} The following analogies between \eqref{eq:z} and \eqref{eq:kv} can be exploited to take the same path as the previous part to show that assumption \ref{ass:c4} holds.
\begin{align*}
z(k,\bar{x})  &\leftrightarrow  k_v(k,\bar{x},\lambda,c) \\
Q(k,\bar{x},\bar{\phi}(k,\bar{x})) &\leftrightarrow \mathscr{K}\left(\bar{x},\bar{\phi}(k,\bar{x}),\rho(\bar{x}),\nu(k,\lambda,c)\right) \\
\mathscr{K}\left(\bar{x},\bar{\phi}(k,\bar{x}),\rho(\bar{x}),\nu(k,\lambda,c)\right) &\leftrightarrow  \mathscr{H}\left(\bar{x},\bar{\phi}(k,\bar{x}),\rho(\bar{x}),\nu(k,\lambda,c),w \right)
\end{align*}

\paragraph*{Assumptions \ref{ass:c5} and \ref{ass:c6}:}
These assumptions are the same as assumption \ref{ass:thm:gamma} in theorem \ref{thm:main}.

\subsection{Convergence Analysis}
Under the regularity conditions mentioned above, the parameter adaptation algorithm \eqref{eq:paa} can be associated with a differential equation that will be derived in this sections.
Suppose the estimate sequence of $\hat{\theta}(k)$ is fixed to a constant value $\hat{\theta}$. Denote $\bar{e}(t,\hat{\theta})$, $\bar{\hat{y}}(t,\hat{\theta})$ and $\bar{\theta}_M(t,\hat{\theta})$ as the (cyclo) stationary processes defined by \eqref{eq:e}, \eqref{eq:yapriori} and \eqref{eq:thetaM}. Note that the stationarity of these processes is admissible only when the closed loop system determined by $\hat{\theta}$ is stable. Suppose $\mathscr{D}_s$ is the set of all values of $\hat{\theta}$ that the stability is attained. The stationary $\tha_D$, by \eqref{eq:integral}, is
\begin{align*}
\bar{\tha}_D(\tha) = \frac{-\alpha}{1-\beta} \hat{D}_B^{-T}(\tha)\tha_M
\end{align*}
where $\hat{D}_B(\tha)$ denotes the value of $\hat{D}_B(k)$ when $\tha(k)=\tha$. Accordingly the control signal associated with $\tha$ is
\begin{align*}
\bar{u}_A(k)= \frac{-\alpha}{1-\beta}\tha_M^T \hat{D}_B^{-1}(\tha)\phi_R(k).
\end{align*}
Therefore, for any fixed $\tha$, the adaptive control algorithm operates in open loop mode and generates a pure feedforward signal. This implies that the closed loop system is stable as long as $\tha_A$ corresponds to an $\hat{A}(\qi)$ polynomial that has all roots strictly inside the unit circle
	\begin{align*}
	\begin{split}
	\mathscr{D}_s:=&\left\{\vphantom{\frac14} \tha:~-\tha_A^T=[\hat{a}_1,\cdots, \hat{a}_{n_A}],\right.\\
	&\qquad \left. {}  1+\hat{a}_1 q +\cdots + \hat{a}_{n_A} q^{{n_A}} =0 \Rightarrow |q|>1 \vphantom{\frac14}\right\}.
	\end{split}
	\end{align*}
This condition is equivalent to assumption \ref{ass:thm:A} in theorem \ref{thm:main}.
The control signal is bounded as long as $\tha_M$ and $\hat{D}_B^{-1}(\tha)\phi_R(k)$ are bounded. The second criterion is equivalent to the condition that $\hat{B}(\qi)$ associated with $\tha_B$ has non-zero magnitude at $\omega_i$'s which is true as long as assumption \ref{ass:thm:B} of theorem \ref{thm:main} holds.
We have
\begin{align*}
\bar{e}(t,\hat{\theta})&=\theta_A \phi_e(t,\hat{\theta}) + \theta_B^T \phi_u(t)+\theta_C^T \phi_{\bar{w}}(t)
\\
&\qquad \qquad \qquad \qquad \qquad   +\bar{\theta}_M^T (t,\hat{\theta}) \phi_R(t)+\bar{w}(t)  \\
\bar{\hat{y}}(t,\hat{\theta})&=\hat{\theta}_A^T \phi_e(t,\hat{\theta}) + \hat{\theta}_B^T \phi_u(t) +\hat{\theta}_C^T \phi_{\epsilon}(t,\hat{\theta}) + \hat{\theta}_M^T {\phi}_R(t,\hat{\theta})
\end{align*}
In the first expression, we have used $w_t(t,\hat{\theta})=0$ since the term $\left(z-1\right)\left[\theta(k)\right]$ in  lemma \ref{lemma:swapping} is zero once $\hat{\theta}(k)$ is frozen. 
The stationary estimation error defined in \eqref{eq:eapriori} is
		\begin{align*}
			&\bar{\epsilon}(t,\tha) = \bar{e}(t,\hat{\theta}) - \bar{\hat{y}}(t,\hat{\theta})\\
			&=\left({\theta}_A^T-\hat{\theta}_A^T\right) \phi_e(t,\hat{\theta}) + \left({\theta}_B^T-\hat{\theta}_B^T\right) \phi_u(t) \\
			&~~~+ \left({\theta}_C^T-\hat{\theta}_C^T\right) \phi_{\epsilon}(t,\hat{\theta}) - \theta_C \phi_{\epsilon}(t,\hat{\theta})+\theta_C^T \phi_{\bar{w}}(t) \\
			&~~~+\bar{\theta}_M^T (t,\hat{\theta}) \phi_R(t)-\hat{\theta}_M^T {\phi}_R(t,\hat{\theta}) + \bar{w}(t)\\
		\end{align*}

By using $\theta_C^T \phi_{\bar{w}}(t)+ \bar{w}(t) = C(\qi)\bar{w}(t)$ and ${\theta}_C^T \phi_{\epsilon}(t,\hat{\theta})+ \bar{\epsilon}(t,\tha)  = C(\qi)\bar{\epsilon}(t,\tha)$
we have
		\begin{align}\label{eq:eps1}
		\begin{split}
			\bar{\epsilon}(t,\tha) &= \frac{1}{C(\qi)}\left[\left({\theta}_A^T-\hat{\theta}_A^T\right) \phi_e(t,\hat{\theta}) + \left({\theta}_B^T-\hat{\theta}_B^T\right) \phi_u(t)\right.\\
			&\left. +  
			 \left({\theta}_C^T-\hat{\theta}_C^T\right) \phi_{\epsilon}(t,\hat{\theta}) +\bar{\theta}_M^T (t,\hat{\theta}) \phi_R(t)-\hat{\theta}_M^T {\phi}_R(t,\hat{\theta})\right] + \bar{w}(t)
			\\
			&=\frac{1}{C(\qi)} \begin{bmatrix} \phi_e(t,\hat{\theta})\\ \phi_u(t)\\ \phi_{\epsilon}(t,\hat{\theta}) \\\phi_R(t) \end{bmatrix}^T
			\begin{bmatrix}
			{\theta}_A-\hat{\theta}_A \\ {\theta}_B-\hat{\theta}_B \\ {\theta}_C-\hat{\theta}_C \\ \bar{\theta}_M(t,\tha) -  \hat{\theta}_M
			\end{bmatrix}+ \bar{w}(t)
		\end{split}
		\end{align}
	
%The scaled rotation matrix $\Delta(\tha)$ satisfies $\hat{\phi}_R(t)=\Delta(\tha){\phi}_R(t,\tha)$.
The stationary process $\bar{\theta}_M(t,\tha)$ can be derived from \eqref{eq:thetaM} and \eqref{eq:integral}
	\begin{align*}\notag
		\theta_M(k+1) &= {D}_B^{T}\tha_D(k+1)+\theta_R \\\notag
		&=\beta {D}_B^{T}\tha_D(k) - \alpha {D}_B^{T}\hat{D}_B^{-T}(k) \tha_M(k)  + \theta_R\\\notag
		%&=\beta \left({D}_B^{T}(k)\tha_D(k) + \theta_R\right)  - \alpha {D}_B^{T}\hat{D}_B^{-T}(k) \tha_M(k)+\left(1-\beta\right) \theta_R \\\notag
		&=\beta \theta_M(k)  - \alpha \Delta^T(\tha) \tha_M(k)+\left(1-\beta\right) \theta_R
	\end{align*}
where $\Delta(\tha)$ is the stationary matrix for $\Delta(k)$ and
	\begin{align*}
		\Delta(k):&= \hat{D}_B^{-1}(k)D_B\\
%		&=\begin{bmatrix}
%		\hat{D}_{B1}^{-1}(k) & 0 & \cdots & 0\\
%		0 & \hat{D}_{B2}^{-1}(k) & \cdots & 0\\
%		\vdots & \vdots &\ddots & \vdots\\
%		0 & 0 & \cdots & \hat{D}_{Bn}^{-1}(k)
%		\end{bmatrix}
%		\begin{bmatrix}
%		{D}_{B1} & 0 & \cdots & 0\\
%		0 & {D}_{B2} & \cdots & 0\\
%		\vdots & \vdots &\ddots & \vdots\\
%		0 & 0 & \cdots & {D}_{Bn}
%		\end{bmatrix}\\
		&=\begin{bmatrix}
		\hat{D}_{B1}^{-1}(k) {D}_{B1} & 0 & \cdots & 0\\
		0 & \hat{D}_{B2}^{-1}(k) {D}_{B2} & \cdots & 0\\
		\vdots & \vdots &\ddots & \vdots\\
		0 & 0 & \cdots & \hat{D}_{Bn}^{-1}(k) {D}_{Bn}
	\end{bmatrix}
	\end{align*}
\begin{align*}
\hat{D}_{Bi}^{-1}(k) {D}_{Bi} &= \left(\frac{1}{\hat{m}_{Bi}} R\left(-\hat{\delta}_{Bi}(k)\right)\right)\left({{m}_{Bi}} R\left(\delta_{Bi}\right)\right)\\
&=\frac{m_{Bi}}{\hat{m}_{Bi}(k)} R(\delta_{Bi}-\hat{\delta}_{Bi}(k))
\end{align*}
Therefore,
\begin{align*}
\bar{\theta}_M(t,\tha) &= \beta \bar{\theta}_M(t,\tha) - \alpha \Delta^T(\tha) \tha_M+\left(1-\beta\right) \theta_R\\
&=\theta_R-\frac{\alpha}{1-\beta}\Delta^T(\tha)\tha_M.
\end{align*}
%Let $\Delta(\tha)$ be a weighted rotation matrix that maps $\hat{\phi}_R(t,\tha)$ to $\phi_R(t)$
%\begin{align*}
%\phi_R(t)=\Delta(\tha)\hat{\phi}_R(t,\tha).
%\end{align*}
Using this definition and the expression for $\bar{\theta}_M$ we have
\begin{align*}
	&\bar{\theta}_M^T (t,\hat{\theta}) \phi_R(t)-\hat{\theta}_M^T {\phi}_R(t) 
	\\ 
	&\qquad \qquad =
	{\phi}_R^T(t)
	\left(I+\frac{\alpha}{1-\beta}\Delta^T(\tha)\right) 
	\left[\theta_M^*-\tha_M\right]
\end{align*}
where
\begin{align}\label{eq:thetaMStar}
\theta_M^* = \left(I+\frac{\alpha}{1-\beta}\Delta(\tha)\right)^{-T}\theta_R.
\end{align}
The expression $I+\frac{\alpha}{1-\beta}\Delta(\tha)$ has singularity point at 
	\begin{align}\label{eq:singularity}
	\begin{split}
		\hat{\delta}_{B_i}&=\delta_{B_i}-\pi\\
		\hat{m}_{B_i}&=\frac{\alpha}{1-\beta}m_{B_i}.
	\end{split}
	\end{align}
By choosing appropriate $\alpha$ and $\beta$ and limiting $\hat{m}_{B_i}$ from above, the singularity point can be avoided. This condition is guaranteed by assumption \ref{ass:thm:B} in theorem \ref{thm:main}. However, as we will see in the sequel, the algorithm avoids such a large phase difference $\delta_{B_i}-\hat{\delta}_{B_i}=\pi$ with probability one even no upper bound is applied to $\hat{m}_{B_i}$.
 
Returning to \eqref{eq:eps1}, we have
	\begin{align}\label{eq:eps2}
	\begin{split}
		& \bar{\epsilon}(t,\tha) =\frac{1}{C(\qi)} 
		\left[\begin{array}{c} \phi_e(t,\hat{\theta})\\ \phi_u(t)\\ \phi_{\epsilon}(t,\hat{\theta}) \\ \hdashline {\phi}_R(t) \end{array}\right]^T
		\times \\
		& \qquad\qquad \left[\begin{array}{c:c} I & 0 \\ \hdashline 0 & I+\frac{\alpha}{1-\beta}\Delta^T(\tha) \end{array}\right]
		\left[\begin{array}{c} {\theta}_A-\hat{\theta}_A \\ {\theta}_B-\hat{\theta}_B \\ {\theta}_C-\hat{\theta}_C \\ \hdashline \theta_M^* -  \hat{\theta}_M \end{array}\right]
	\end{split}
	\end{align}
When $\Delta$ is bounded, by choosing $\beta$ close enough to 1 and $\alpha \gg 1-\beta$ the inverse term is not subjected to numerical issues and $\theta_M^* \ll \theta_R$.

Introduce 

	\begin{widetext}
			\begin{subequations}\label{eq:G-all}
				\begin{align}
				\label{eq:Gtilde}
				\tilde{G}(\tha) 
				: &=
				\frac{1}{t}\sum\limits_{k=1}^{t} \left(
				\left[\begin{array}{c} \phi_e(k,\hat{\theta})\\ \phi_u(k)\\ \phi_{\epsilon}(k,\hat{\theta}) \\{\phi}_R(k) \end{array}\right]
				\left[\begin{array}{c:c}    \frac{1}{C(\qi)} & 0 \\ \hdashline  0 & \frac{1+H(q^{-1};\tha)}{C(\qi)}  \end{array}\right]
				\left[\begin{array}{c} \phi_e(k,\hat{\theta})\\ \phi_u(k)\\ \phi_{\epsilon}(k,\hat{\theta}) \\ {\phi}_R(k) \end{array}\right]^T\right)
				\\
				\label{eq:G}
				G(\tha):&= \frac{1}{t}\sum\limits_{k=1}^{t} 
				\left[\begin{array}{c} \phi_e(k,\hat{\theta})\\ \phi_u(k)\\ \phi_{\epsilon}(k,\tha)\end{array} \right]
				\\
				\label{eq:gsmall}
				g(\tha):&=\frac{1}{t}\sum\limits_{k=1}^{t} {\phi}_R^T(k){\phi}_R(k)
				\end{align}
			\end{subequations}
	\end{widetext}
and decompose $\phi_e(k)$ to a stochastic and deterministic part as $\phi_e(k)=\phi_{ed}(k)+\phi_{es}(k)$. The fact that all stochastic processes are zero mean along with \eqref{eq:sumToExpect} imply
	\begin{widetext}
			\begin{align}
			\tilde{G}(\tha)& \rightarrow \tilde{G}_s(\tha)+\tilde{G}_d(\tha) \qquad \text{w.p. 1 as }t\rightarrow \infty
			\\
			\tilde{G}_s(\tha)&:=\E \left(
			\begin{bmatrix} \phi_{es}(k,\hat{\theta})\\ 0\\ \phi_{\epsilon}(k,\hat{\theta}) \\0 \end{bmatrix}
			\frac{1}{C(\qi)} 
			\begin{bmatrix} \phi_{es}(k,\hat{\theta})\\ 0\\ \phi_{\epsilon}(k,\hat{\theta}) \\ 0 \end{bmatrix}^T\right)
			\\
			\tilde{G}_d(\tha)&:=\frac{1}{t}\sum\limits_{k=1}^{t} \left(
			\begin{bmatrix} \phi_{ed}(k,\hat{\theta})\\ \phi_u(k)\\ 0 \\ \hdashline  {\phi}_R(k) \end{bmatrix}
			\left[\begin{array}{c:c}    \frac{1}{C(\qi)} & 0 \\ \hdashline  0 & \frac{1+H(q^{-1};\tha)}{C(\qi)}  \end{array}\right]
			\begin{bmatrix} \phi_{ed}(k,\hat{\theta})\\ \phi_u(k)\\ 0 \\ \hdashline {\phi}_R(k) \end{bmatrix}^T\right)
			\end{align}
	\end{widetext}
	
Here, $H(\qi, \tha)$ is a stable and causal transfer function, e.g. an FIR LTI system, that at $\omega_i$'s has magnitude and phase responses equal to the corresponding magnitudes and phases in $ \frac{\alpha}{1-\beta}\Delta^T(\tha)$. It is trivial that such an LTI transfer function can be found for any $\Delta^T(\tha)$ by considering at most $2n$ coefficients.

Under the regularity conditions and conditions on the stochastic processes $\bar{w}(k)$ and $u(k)$ that were mentioned above the parameter adaptation algorithm in \eqref{eq:paa} can be associated with the differential equation \cite{ljung1977analysis}
\begin{subequations}\label{eq:ode}
\begin{align}\label{eq:ode-theta}
\frac{d}{dt}\hat{\theta}(t)&=\bm{cc} F^{-1}(t) & 0 \\ 0 & f^{-1}(t)I \mb 
\tilde{G}(\tha(t))
%\left[\begin{array}{c:c} I & 0 \\ \hdashline 0 & \frac{\alpha}{1-\beta}I+\Delta^T(\tha) \end{array}\right]
\begin{bmatrix} {\theta}_A-\hat{\theta}_A \\ {\theta}_B-\hat{\theta}_B \\ {\theta}_C-\hat{\theta}_C \\ \theta_M^* -  \hat{\theta}_M \end{bmatrix}
\\ 
\label{eq:ode-F}
\frac{d}{dt} F(t)&=G(\tha(t))-F(t)
\\
\label{eq:ode-f}
\frac{d}{dt} f(t)&=g(\tha(t))-f(t).
\end{align}
\end{subequations}
Moreover, the convergence point(s) of parameter adaptation algorithm \eqref{eq:paa} can be related to the set of stationary points, say $\mathscr{D}_c$, of the differential equations \eqref{eq:ode} through corollary 1 in \cite{ljung1977analysis}. The following conditions, that are already shown to be satisfied partially, are required to use the corollary results
\begin{itemize}
	\item 
	Regularity conditions mentioned above should be satisfied.
	\item
	$\tha(k) \in \mathscr{D}_s$ infinitely often with probability one.
	\item
	$\|{\phi}(k)\|$ is bounded infinitely often whenever $\tha(k)$ belongs to $\mathscr{D}_s$
	\item
	There is a Lyapunov function $V\left(\tha(t), F(t), f(t)\right)$ such that 
	\begin{align*}
	\frac{d}{dt} V\left(\tha(t), F(t), f(t)\right)&\le 0 \quad \text{for  }\tha(t)\in \mathscr{D}_s,~F(t)>0,~f(t)>0\\
	\frac{d}{dt} V\left(\tha(t), F(t), f(t)\right)&= 0 \quad \text{for  }\tha(t)\in \mathscr{D}_c
	\end{align*}
\end{itemize}
We have already shown that the first condition is satisfied  when a projection scheme is considered. The third condition can be satisfied by restricting $\tha_B(k)$ to
\begin{align*}
\mathscr{D}_B:=
\left\{\vphantom{\frac12}  \tha_B : |b_1^i e^{-j\omega_m} + \cdots + b_{n_A}^i  e^{-jn_A \omega_m}|>0  \right. \\
\left. \forall i \in \{1,\ldots, n_i\} \text{  and  } \forall m \in \{1,\ldots,n\} \vphantom{\frac12}  \right\}.
\end{align*}
This means that the magnitude of $\hat{B}(\qi;k)$ at excitation frequencies should be bounded  from below by a small positive value. This is equivalent to assumption \ref{ass:thm:B} in theorem \ref{thm:main}. In case $\tha_B(k)$ does not belong to $\mathscr{D}_B$, the parameters can be projected to $\mathscr{D}_B$ by scaling $\tha_B(k)$.
%This results in boundness of ${\phi}_R(k)$ and accordingly $\hat{\phi}(k)$. 
An implication of this restriction is that $\Delta(\tha(k))$ is also always bounded. 
%This is a useful fact for the last condition because the term $\frac{\alpha}{1-\beta}I+\Delta^T(\tha)$ will be positive definite by choosing $\beta$ close (from left) enough to 1. 

Analogous to \cite{ljung1977positive} an admissible Lyapunov function can be defined when $\tilde{G}(\tha)+\tilde{G}^T(\tha)$ is positive definite. This is possible when both $\frac{1}{C(\qi)}$ and $\frac{H(\qi,\tha)}{C(\qi)}$ are strictly positive real. The second condition can be relaxed further since the response of $H(\qi; \tha)$ is only important at $\omega_i$'s. Therefore, $\tilde{G}(\tha)+\tilde{G}^T(\tha)$ is positive definite if
\begin{enumerate}
	\item $\phi_u$ is persistently exciting of order $2n$.
	\item $\frac{1}{C(\qi)}$ is strictly positive real (SPR).
	\item Absolute phase of $\frac{H(e^{-j\omega_i}; \tha)}{C(e^{-j \omega_i})}$ is less than $90$ degrees.
\end{enumerate}
%The third condition can be justified by comparing \eqref{eq:Gtilde} with
%\begin{align*}
%\left[\begin{array}{c} \phi_1\\ \phi_2\end{array}\right]
%\left[\begin{array}{cc}    \frac{1}{C} & 0 \\   0 & \frac{1+H}{C}  \end{array}\right]
%\left[\begin{array}{c} \phi_1\\ \phi_2\end{array}\right]^T 
%&= 
%\left[\begin{array}{c} \phi_1\\ \phi_2\end{array}\right]
%\frac{1}{C}
%\left[\begin{array}{c} \phi_1\\ \phi_2\end{array}\right]^T
%+
%\left[\begin{array}{cc}    0 & 0 \\   0 & \phi_2 \frac{H}{C}\phi_2^T  \end{array}\right].
%\end{align*}
%If $1/C(\qi)$ is strictly positive real, the first term on the left will make a positive definite matrix when it is summed with its transpose. Similarly, when $H(\qi)/C(\qi)$ is SPR, summation of the second term with its transpose results in a positive semi-definite matrix. This implies that the summation of the two transfer functions results in a positive definite matrix when condition 2 and 3 hold.
%
Note that these conditions are equivalent to assumptions \ref{ass:thm:u},\ref{ass:thm:C} and \ref{ass:thm:H} of theorem \ref{thm:main} respectively.

\begin{proof}[Theorem \ref{thm:main}]
Theorem 2 in \cite{ljung1977analysis} implies that the convergence point(s) of the parameter adaptation algorithm \eqref{eq:paa} are among the stable  stationary points of \eqref{eq:ode}. For an SPR $1/C(\qi)$, the cross covariance matrix 
\begin{align*}
\frac{1}{t}\sum\limits_{k=1}^{t} \left(
\left[\begin{array}{c} \phi_e(k,\hat{\theta})\\ \phi_u(k)\\ \phi_{\epsilon}(k,\hat{\theta}) \\{\phi}_R(k) \end{array}\right]
\frac{1}{C(\qi)}
\left[\begin{array}{c} \phi_e(k,\hat{\theta})\\ \phi_u(k)\\ \phi_{\epsilon}(k,\hat{\theta}) \\ {\phi}_R(k) \end{array}\right]^T\right)
\end{align*}
added to its transpose makes a positive definite matrix. Therefore, from \eqref{eq:eps2}, the only stationary point of \eqref{eq:ode-theta} is given by
\begin{align*}
\left[\begin{array}{c:c} I & 0 \\ \hdashline 0 & I+\frac{\alpha}{1-\beta}\Delta^T(\tha) \end{array}\right]
\left[\begin{array}{c} {\theta}_A-\hat{\theta}_A \\ {\theta}_B-\hat{\theta}_B \\ {\theta}_C-\hat{\theta}_C \\ \hdashline \theta_M^* -  \hat{\theta}_M \end{array}\right]\
=0.
\end{align*}
The left matrix singularity points are described in \eqref{eq:singularity}. It is trivial that the parameter $\hat{\theta}_B$ corresponding to such a singularity point does not fall in the null space of the left matrix. 
Hence, the only stationary point of \eqref{eq:ode} is
	\begin{align*}
		\theta^*
		=
		\left[\begin{array}{c} \hat{\theta}_A \\ \hat{\theta}_B \\ \hat{\theta}_C \\  \hat{\theta}_M \end{array}\right]
		=
		\left[\begin{array}{c} {\theta}_A \\ {\theta}_B\\ {\theta}_C\\ \frac{1-\beta}{1-\beta+\alpha} \theta_R \end{array}\right] 
	\end{align*} 
where the last term comes from \eqref{eq:thetaMStar} when $\tha_B=\theta_B$.
Moreover, it can be shown that this is a locally stable stationary point. 
Suppose $\B(\theta_B,\rho(\theta_B))$ be a neighborhood of $\theta_B$ in which $|\delta_{B_i}-\hat{\delta}_{B_i}|<90$. The quadratic function
\begin{align*}
V(\tha):=\tha^T\left(\tilde{G}(\tha)+\tilde{G}^T(\tha)\right)\tha.
\end{align*}
is positive definite and has negative definite Lie derivative along \eqref{eq:ode} trajectories as long as $\tha \in \B(\theta^*,\rho(\theta_B))$. 
This is because  $\|\theta_B-\tha_B\|\le \|\theta^*-\tha\|$ implies that starting the trajectory from $\tha(0) \in \B(\theta^*,\rho(\theta_B))$, the estimated $\tha_B$ always stays in a neighborhood with a smaller radius around $\theta_B$. Therefore, decreasing $\|\theta^*-\tha\|$ results in keeping $\tha_B$ in $\B(\theta^*,\rho(\tha_B))$ which itself implies more reduction in  $\|\theta^*-\tha\|$.
Accordingly, $V(\tha)$ is a Lyapunov function for \eqref{eq:ode} and the equilibrium state $\theta^*$ is stable in the sense of Lyapunov.

\end{proof}
\begin{proof}[Theorem \ref{lemma:usingCbar}]
	The proof of theorem \ref{lemma:usingCbar} is similar to the proof of theorem \ref{thm:main} up to equation \eqref{eq:eps2}. 
	Starting from \eqref{eq:G-all}, one needs to substitute all instances of $C(\qi)$ by $C(\qi)/\bar{C}(\qi)$ to show the results.
\end{proof}

\begin{proof}[Theorem \ref{thm:main2}]
	The proof is based on to the proof of theorem \ref{thm:main}.	
	When there is no prior knowledge regarding $B(\qi)$ in hand, it may not be possible to set the initial conditions of \eqref{eq:paa} and accordingly \eqref{eq:ode} to guarantee SPR condition on $H(\qi; \tha)/C(\qi)$ term. However, the region of attraction for differential equation \eqref{eq:ode} can be enlarged in practice by increasing the excitation energy. Consider the upper states of \eqref{eq:ode-theta} 
	
	\begin{widetext}
		\begin{align}\label{eq:paa_ode_upperpart}
		\begin{split}
		\frac{d}{dt}\begin{bmatrix} \hat{\theta}_A \\ \hat{\theta}_B \\ \hat{\theta}_C \end{bmatrix}&=F^{-1}(t)
		\frac{1}{t}
		\sum\limits_{k=1}^{t} \left(
		\left[\begin{array}{c} \phi_e(k,\hat{\theta})\\ \phi_u(k)\\ \phi_{\epsilon}(k,\hat{\theta})  \end{array}\right]
		\frac{1}{C(\qi)} 
		\left[\begin{array}{c} \phi_e(k,\hat{\theta})\\ \phi_u(k)\\ \phi_{\epsilon}(k,\hat{\theta})  \end{array}\right]^T\right)
		\begin{bmatrix} {\theta}_A-\hat{\theta}_A \\ {\theta}_B-\hat{\theta}_B \\ {\theta}_C-\hat{\theta}_C  \end{bmatrix}
		\\
		&\qquad \qquad\qquad\qquad\qquad\qquad\qquad 
		+F^{-1}(t)\frac{1}{t}
		\sum\limits_{k=1}^{t} 
		\left[\begin{array}{c} \phi_e(k,\hat{\theta})\frac{1+H(\qi; \tha)}{C(\qi)} \phi_R^T(k)\\ 0\\ 0  \end{array}\right]
		\theta_M^* -  \hat{\theta}_M
		\end{split}
		\end{align}
	\end{widetext}
	when $1/C(\qi)$ is SPR, the first term on the right attracts the states to $\begin{bmatrix}\theta_A^T & \theta_B^T & \theta_C^T\end{bmatrix}^T$. However, the second term might be repulsive when $H(\qi; \tha)/C(\qi)$ is not SPR. 
	 In \eqref{eq:paa_ode_upperpart}, the second term on the right hand side is 
	 bounded when assumption \ref{ass:thm2:thetabounded} in theorem \ref{thm:main2} holds true. As a result, by increasing $\alpha_{dc}$ the attraction of the first term increases which can lead to bringing $\tha_B$ into $\mathscr{D}_B$ when $\alpha_{dc}$ is chosen large enough.  
	 This means that by choosing enough excitation in such a case, the convergence rate of the first term can be increased such that the first term brings $\tha_B$ into a vicinity of $\theta_B$ in which the second term is also attractive.
\end{proof}
